# Supplementary material for: DITRON: Distributed Multi-level Tiling Compiler for Parallel Tensor Programs
Source: arXiv:2605.02953 source file (2026-05-02)
Supplement: Supplementary file 1 [file appendix.tex]

\section{Hello World}
%\subsection{Hello World}
